# Supplementary material for: Quantitative predictions of the thermal conductivity in transition metal dichalcogenides: The impact of point defects in MoS$_2$ and WS$_2$ monolayers
Source: arXiv:2310.09405 ancillary file (2023-10-13)
Supplement: Supplementary file 1 [file supplemental-material.pdf]

# Supplemental Material

## Quantitative predictions of the thermal conductivity in transition metal dichalcogenides: The impact of point defects in $MoS_2$ and $WS_2$ monolayers

Srinivisan Mahendran[1], Jesús Carrete[2], Andreas Isacsson[1], Georg K. H. Madsen[2], and Paul Erhart[1,*]

[1] *Department of Physics, Chalmers University of Technology, SE-41296, Gothenburg, Sweden*
[2] *Institute of Materials Chemistry, TU Wien, A-1060 Vienna, Austria*
[*] *erhart@chalmers.se*

# Contents

**Supplemental Tables** **2**
S1. Computational parameters . . . . . . . . . . 2

**Supplemental Figures** **3**
S1. Lattice thermal conductivity of $WS_2$ in the presence of S vacancies . . . . . . 3
S2. Lattice thermal conductivity of $MoS_2$ and $WS_2$ as a function of defect concentration . . . 3
S3. Phonon dispersion relations for $MoS_2$ with defect scattering rates . . . . . . 4
S4. Phonon dispersion relations for $WS_2$ with defect scattering rates . . . . . . 4

**Supplemental References** **5**

# Supplemental Tables

Table S1: **Computational parameters.** Summary of parameters used for extraction of the second-order FCs of $MoS_2$ defect supercells. $N_{par}$: Total number of parameters; $N_{non\text{-}zero}$: Number of non-zero parameters; RMSE: root-mean-square error over training (t) and validation (v) sets in meV $Å^{-1}$.

| Defect | $N_{par}$ | $N_{non\text{-}zero}$ | RMSE(t) | RMSE(v) |
|---|---|---|---|---|
| $S_{vac}$ | 7933 | 5714 | 1.6 | 2.3 |
| $S_{divac}$ | 23 367 | 4687 | 7.4 | 10.0 |
| $S_{divac-z}$ | 4064 | 3254 | 4.3 | 5.1 |
| $S_{ad}$ | 8043 | 6759 | 1.4 | 2.1 |
| $K_{ad-1}$ | 8030 | 5783 | 2.2 | 3.1 |
| $K_{ad-2}$ | 8028 | 4818 | 2.3 | 3.2 |
| $Li_{ad-1}$ | 8054 | 6122 | 2.4 | 3.6 |
| $Li_{ad-2}$ | 8052 | 6764 | 2.0 | 3.0 |
| $Mo_{vac}$ | 4049 | 3888 | 1.8 | 2.2 |
| $Na_{ad-1}$ | 8045 | 6440 | 1.9 | 2.8 |
| $Na_{ad-2}$ | 8043 | 5475 | 1.9 | 2.7 |

# Supplemental Figures

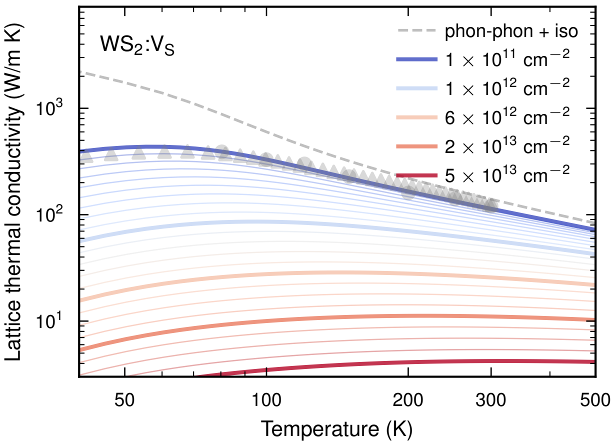


Figure S1: **Lattice thermal conductivity of $WS_2$ in the presence of S vacancies.** Temperature dependent experimental data from Jiang *et al.* (circles; Ref. 1) and Pisoni *et al.* (triangles; Ref. 2).

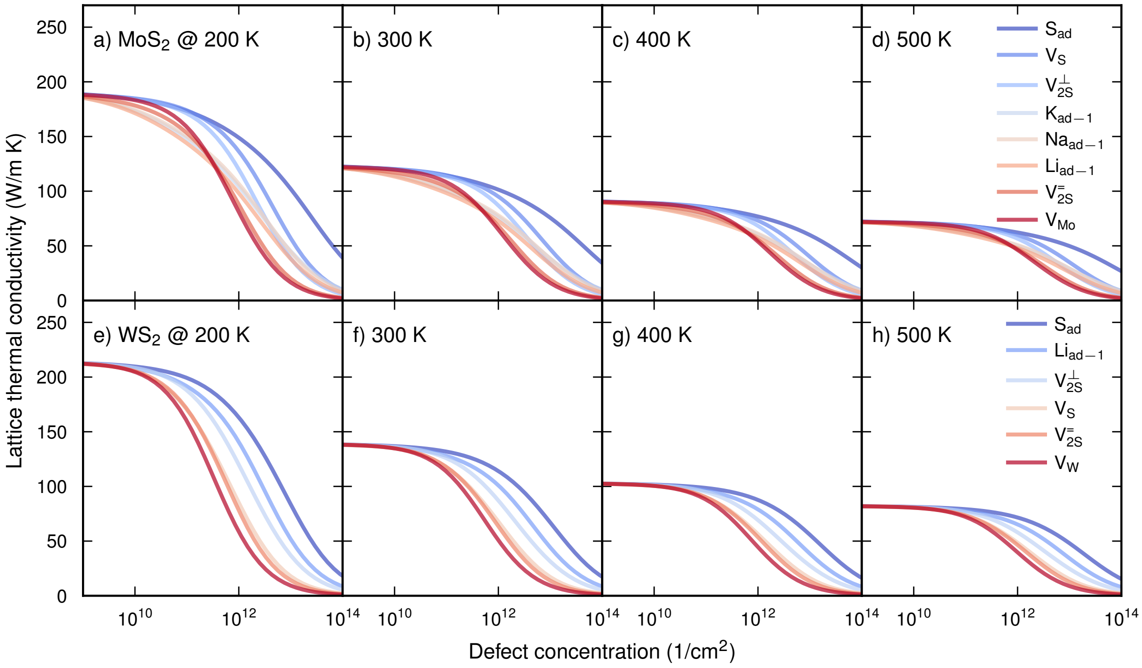


Figure S2: **Lattice thermal conductivity of $MoS_2$ and $WS_2$ as a function of defect concentration.**

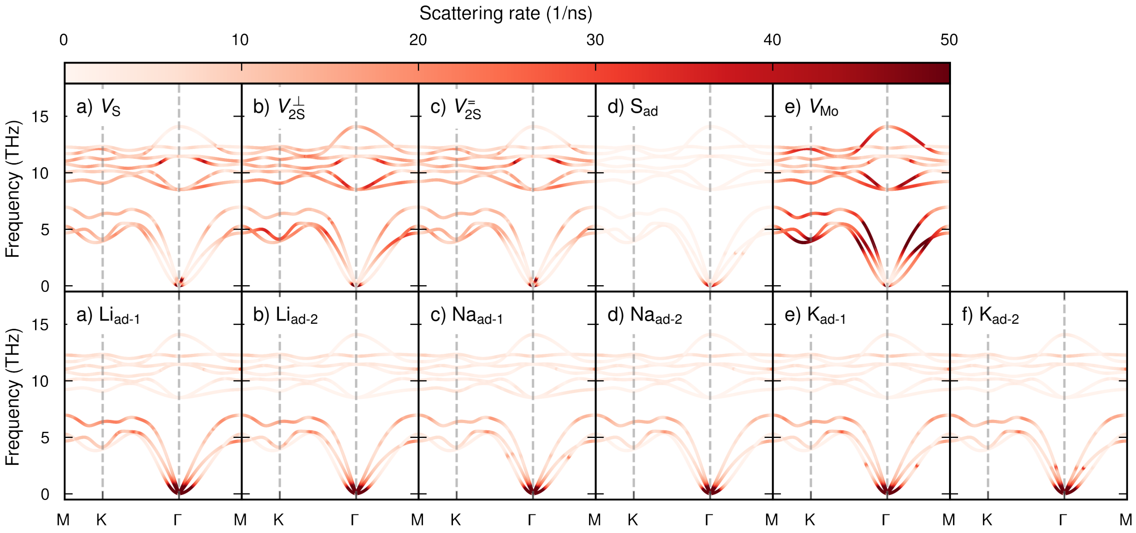


Figure S3: **Phonon dispersion relations for $MoS_2$ with defect scattering rates.** The scattering rates are shown for a concentration of 1 defect per $10^3$ unit cells (approximately $10^{11}$ cm$^{-2}$).

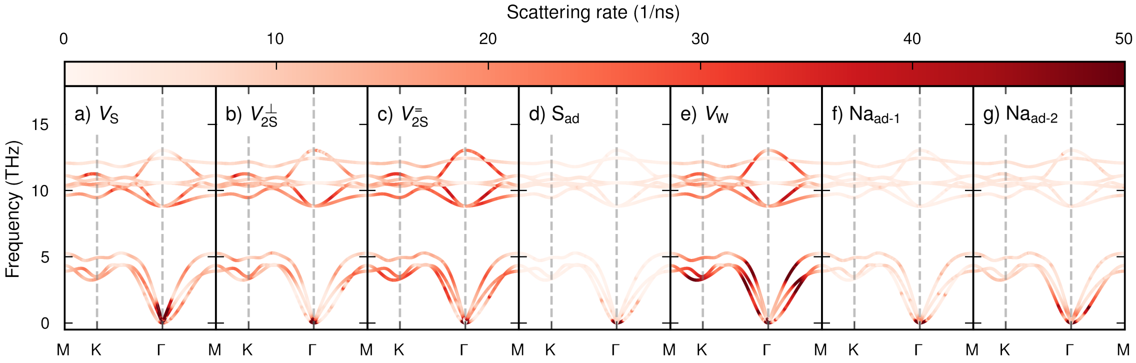


Figure S4: **Phonon dispersion relations for $WS_2$ with defect scattering rates.** The scattering rates are shown for a concentration of 1 defect per $10^3$ unit cells (approximately $10^{11}$ cm$^{-2}$).

## Supplemental References


(1) Jiang, P.; Qian, X.; Gu, X.; Yang, R. *Advanced Materials* **2017**, *29*, 1701068, DOI: 10.1002/adma.201701068.

(2) Pisoni, A.; Jacimovic, J.; Gaál, R.; Náfrádi, B.; Berger, H.; Révay, Z.; Forró, L. *Scripta Materialia* **2016**, *114*, 48–50, DOI: 10.1016/j.scriptamat.2015.11.028.
